# Supplementary material for: Robot Task Planning and Situation Handling in Open Worlds
Source: arXiv:2210.01287 source file (2024-09-29)
Supplement: Supplementary file 1 [file appendix.tex]

\newpage
\appendix

\section{Questionnaire for Collecting Situation Dataset}
To collect execution-time situations, a questionnaire was designed and published on Amazon Mechanical Turk.
Fig.~\ref{fig:questionnaire} shows the Mechanical Turk interface for one everyday task (i.e., drinking water).
In the interface, each MTurker was provided with a task description, including steps for completing the task.
The MTurkers were asked to respond to a questionnaire by identifying one step in the provided plan and describing a situation that might occur in that step within the blank.
On the questionnaire, there are 12 everyday tasks (e.g., setting a dining table) associated with their steps, which were extracted from an existing dataset~\cite{huang2022language}.
In the end, we have collected a dataset of 1128 valid situations, where each instance of the dataset corresponds to a situation that prevents a service robot from completing a task in a dining domain. 
In the next section, we will discuss the statistics of the dataset.

% editable figure link: https://docs.google.com/drawings/d/1XGV3-0wbz_E_x3a2IkxKsxvq6dRzHu2mC6bA4e18FXA/edit
\begin{figure}[!hpt]
\centering
\includegraphics[width=0.9\columnwidth]{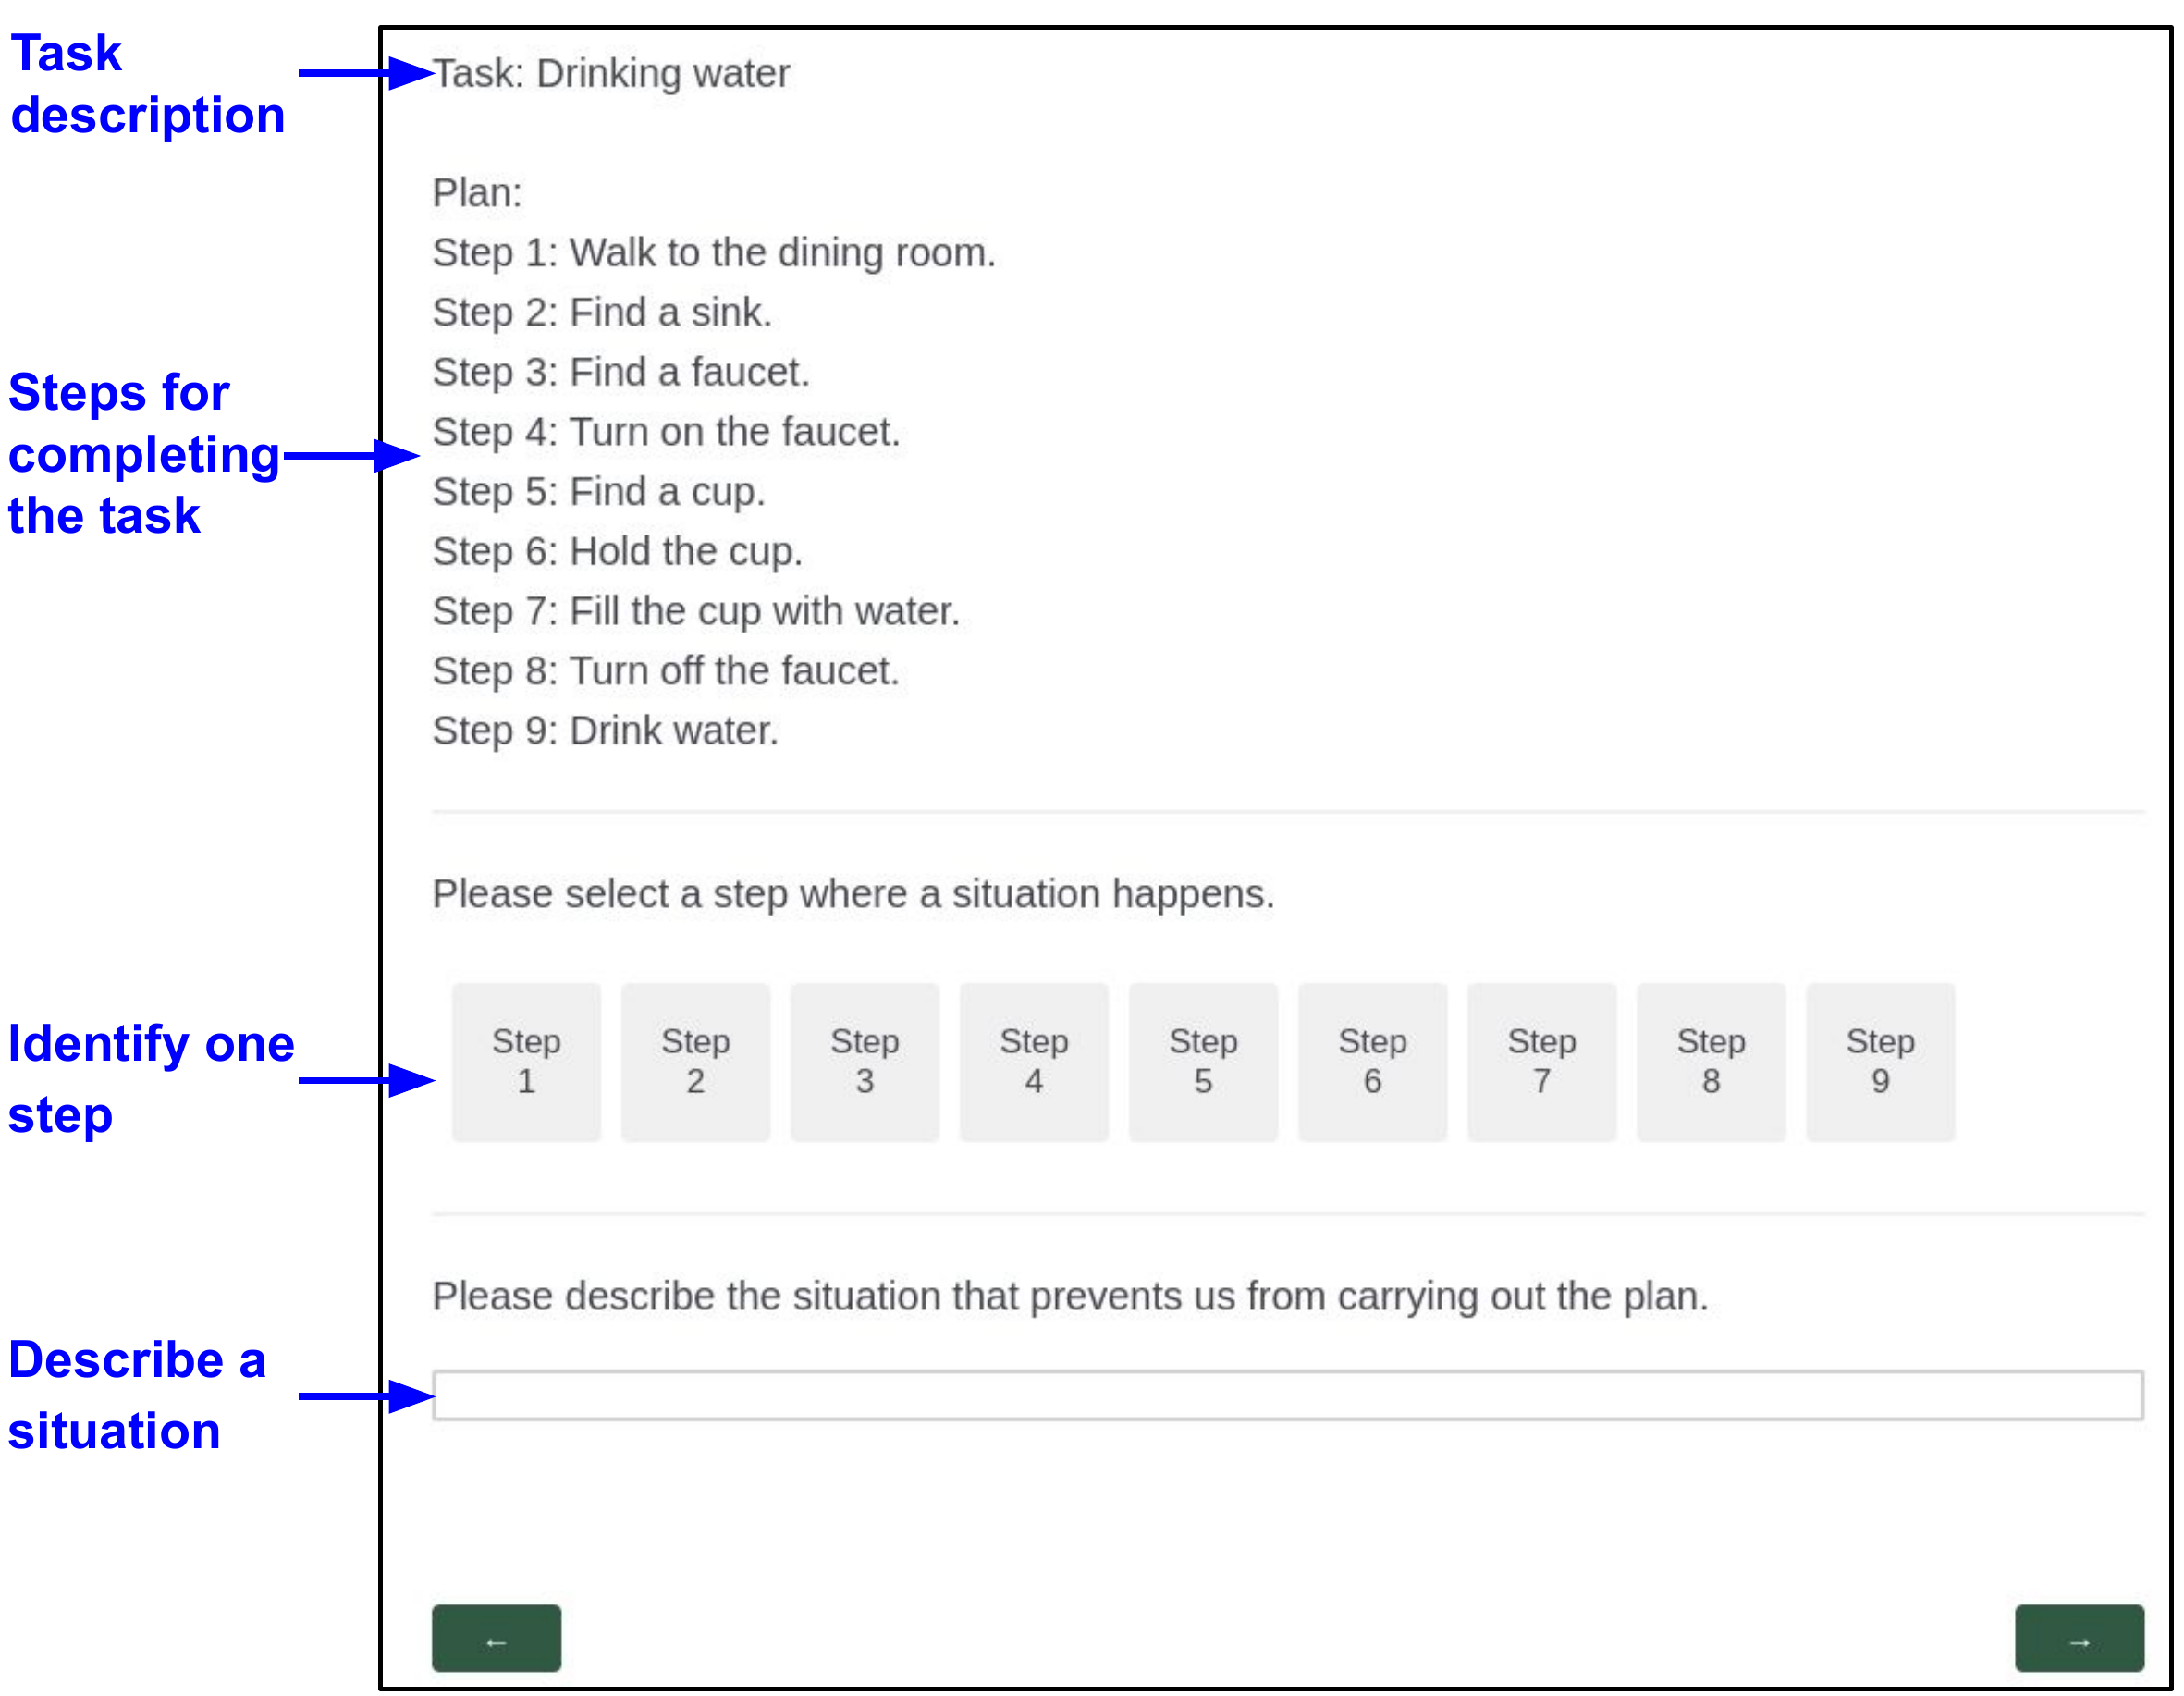}
\caption{The Mechanical Turk interface for the task of drinking water.
Each MTurker was provided with a task description, including nine steps for completing the task. 
The MTurkers were asked to respond to a questionnaire by identifying one step (from Steps 1 to 9) in the provided plan and describing a situation that might occur in that step.
}\label{fig:questionnaire}
\end{figure}

\section{Statistics of Situation Dataset}
Figs.~\ref{fig:situation123} and~\ref{fig:situation456} show the statistics of situations for six everyday tasks used in our evaluation, where \textit{x-axis} reflects the occurrence of each \textit{distinguishable situations}, and \textit{y-axis} represents each distinguishable situations, respectively.
In the top left corner of each subfigure, (X) represents the number of distinguishable situations in each task.
In the bottom right corner of each subfigure, Total = X represents the number of \textit{situations} in each task.
According to the two figures, we can see that there are at least 92 situations collected for each of the six tasks used in our evaluation, with 16 to 22 distinguishable situations.

% editable figure: https://docs.google.com/drawings/d/16Eq8cAv7o8NCepNjZRsYNYYrCZU9MFdpxel-CryJGpg/edit
\begin{figure}[!hpt]
\centering
\includegraphics[width=1\columnwidth]{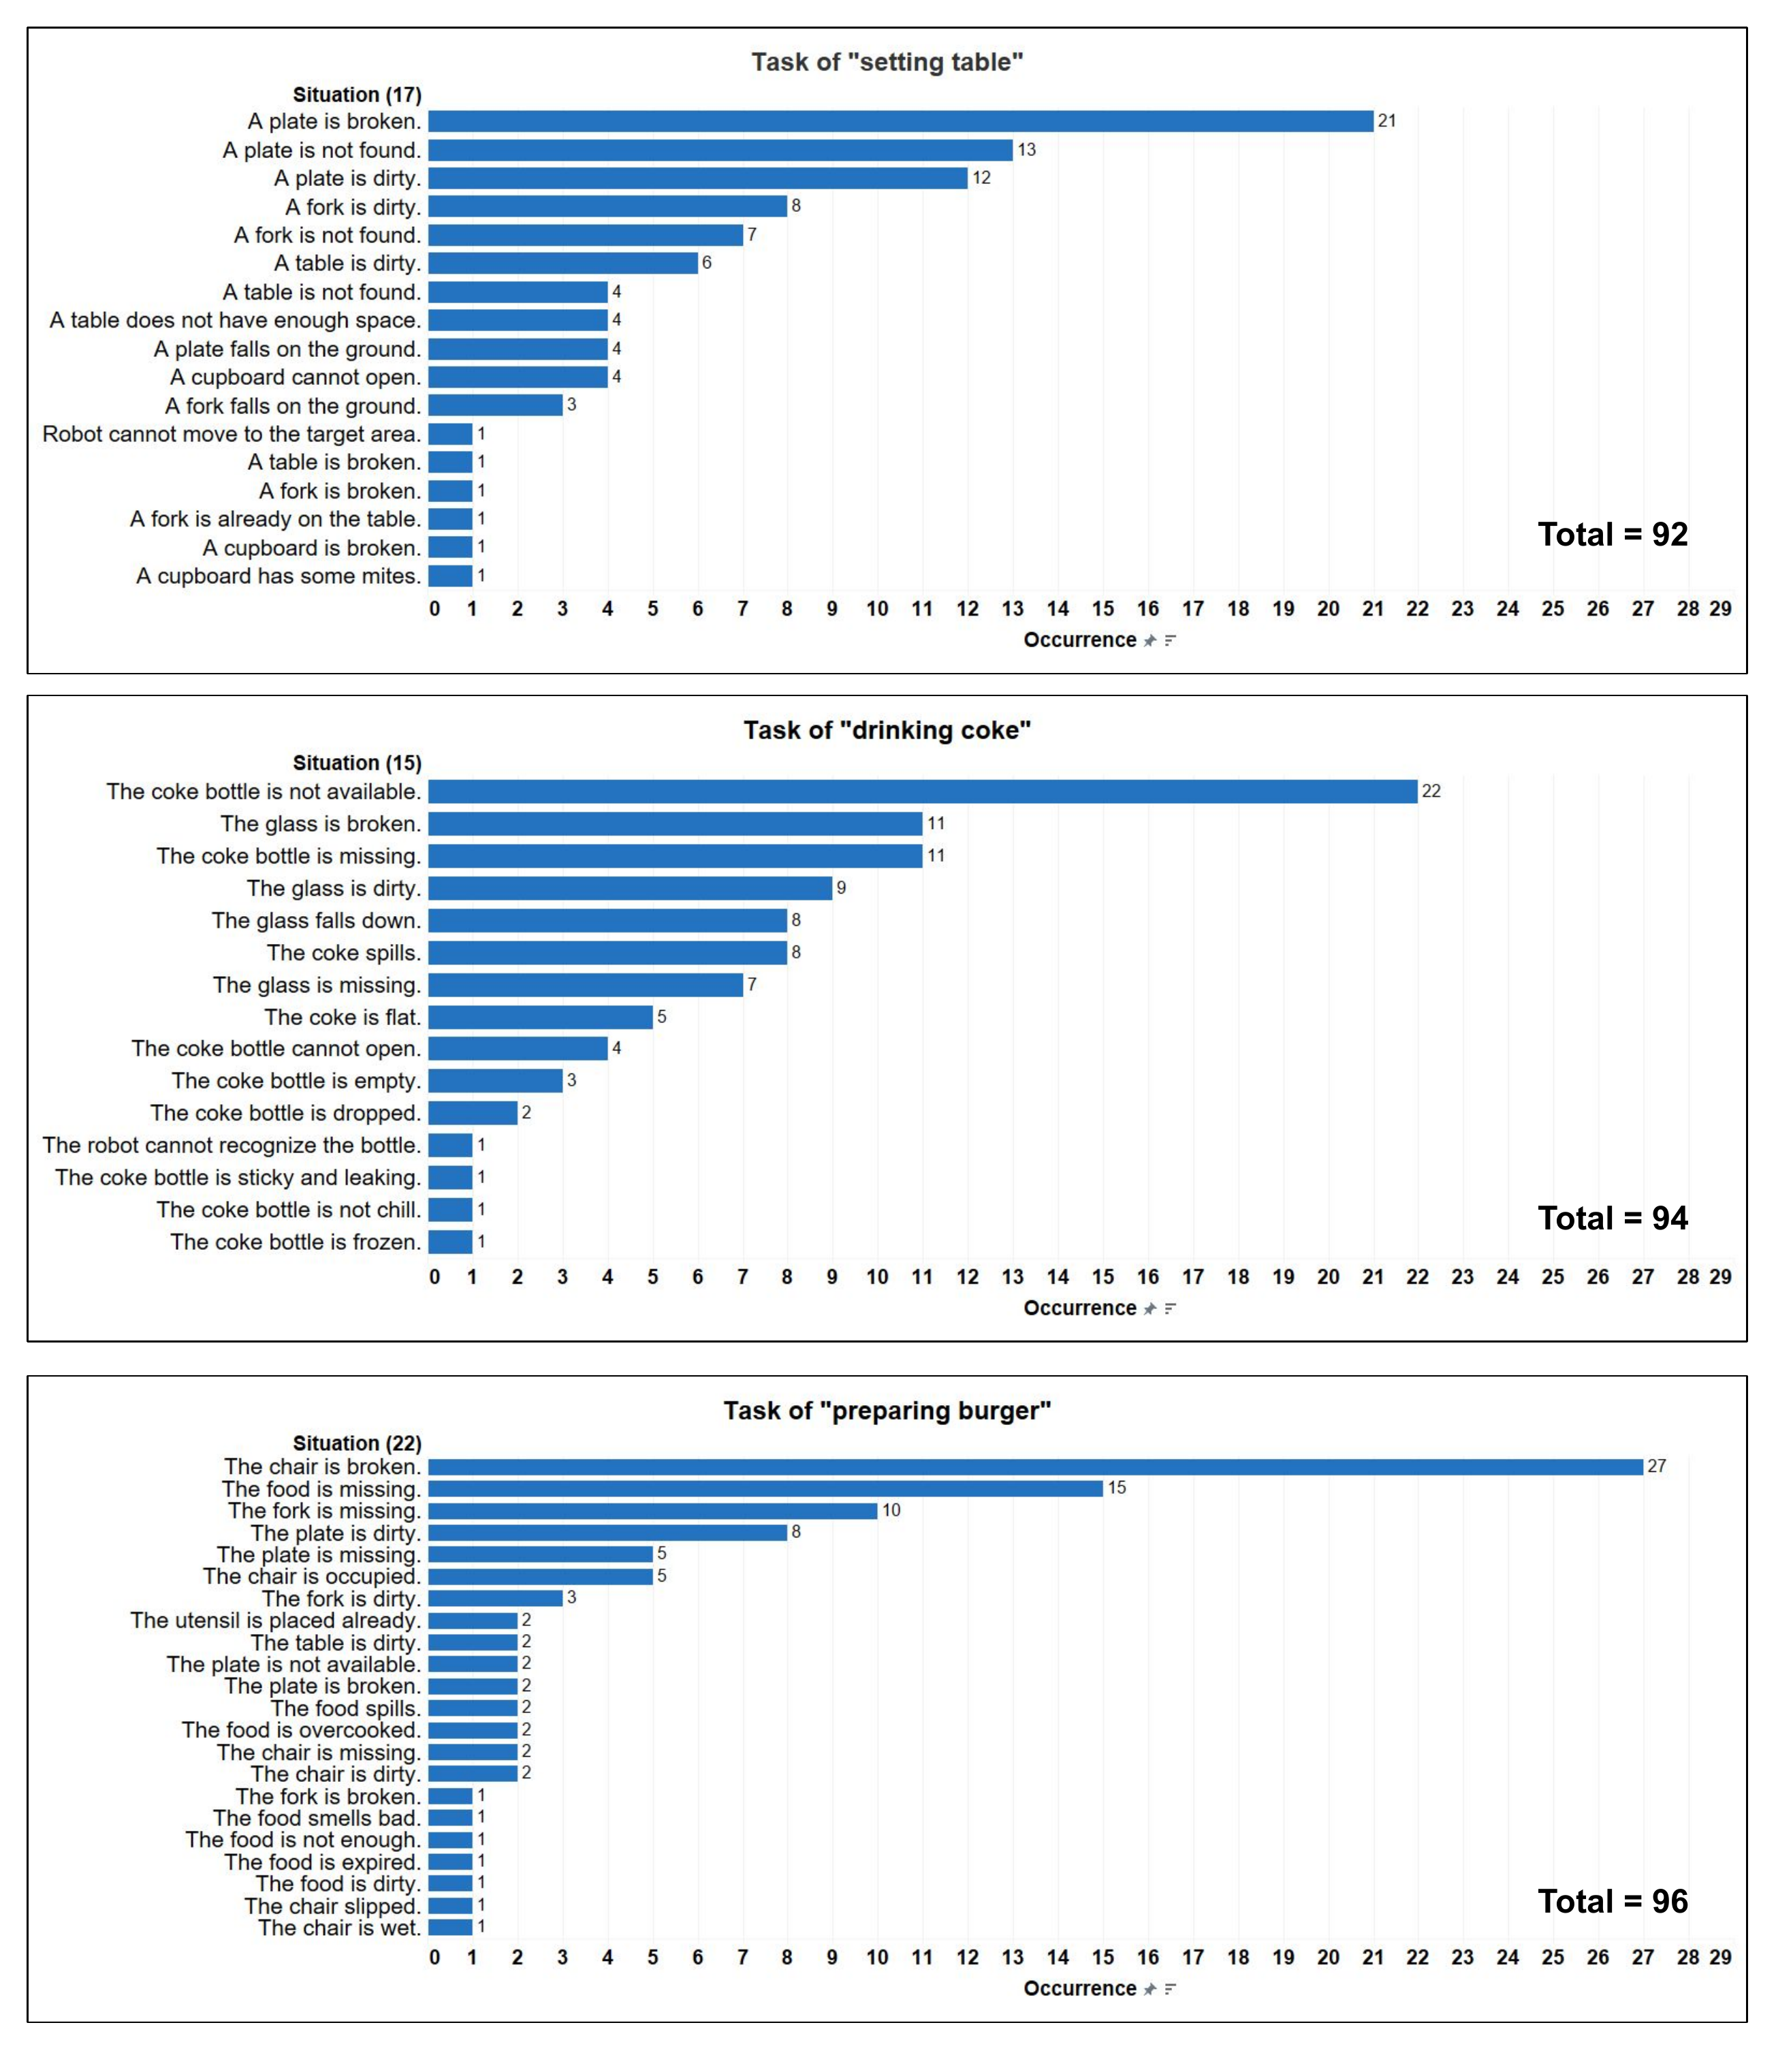}
\caption{
\textbf{Top:} Details of situations in the task of ``setting table'';
\textbf{Middle:} Details of situations in the task of ``drinking coke'';
\textbf{Bottom:} Details of situations in the task of ``preparing burger'';
\textit{x-axis} reflects the occurrence of each \textit{distinguishable situations}, and \textit{y-axis} represents each distinguishable situations, respectively.
(X) in the top left corner of each subfigure represents the number of distinguishable situations in each task.
Total = X indicates the number of situations in each task.
}\label{fig:situation123}
\end{figure}

% editable figure: https://docs.google.com/drawings/d/1xJtnax8bofkahmUos5tetZ_9kZLNtT2KkIzmzt9Irw0/edit
\begin{figure}[t]
\centering
\includegraphics[width=1\columnwidth]{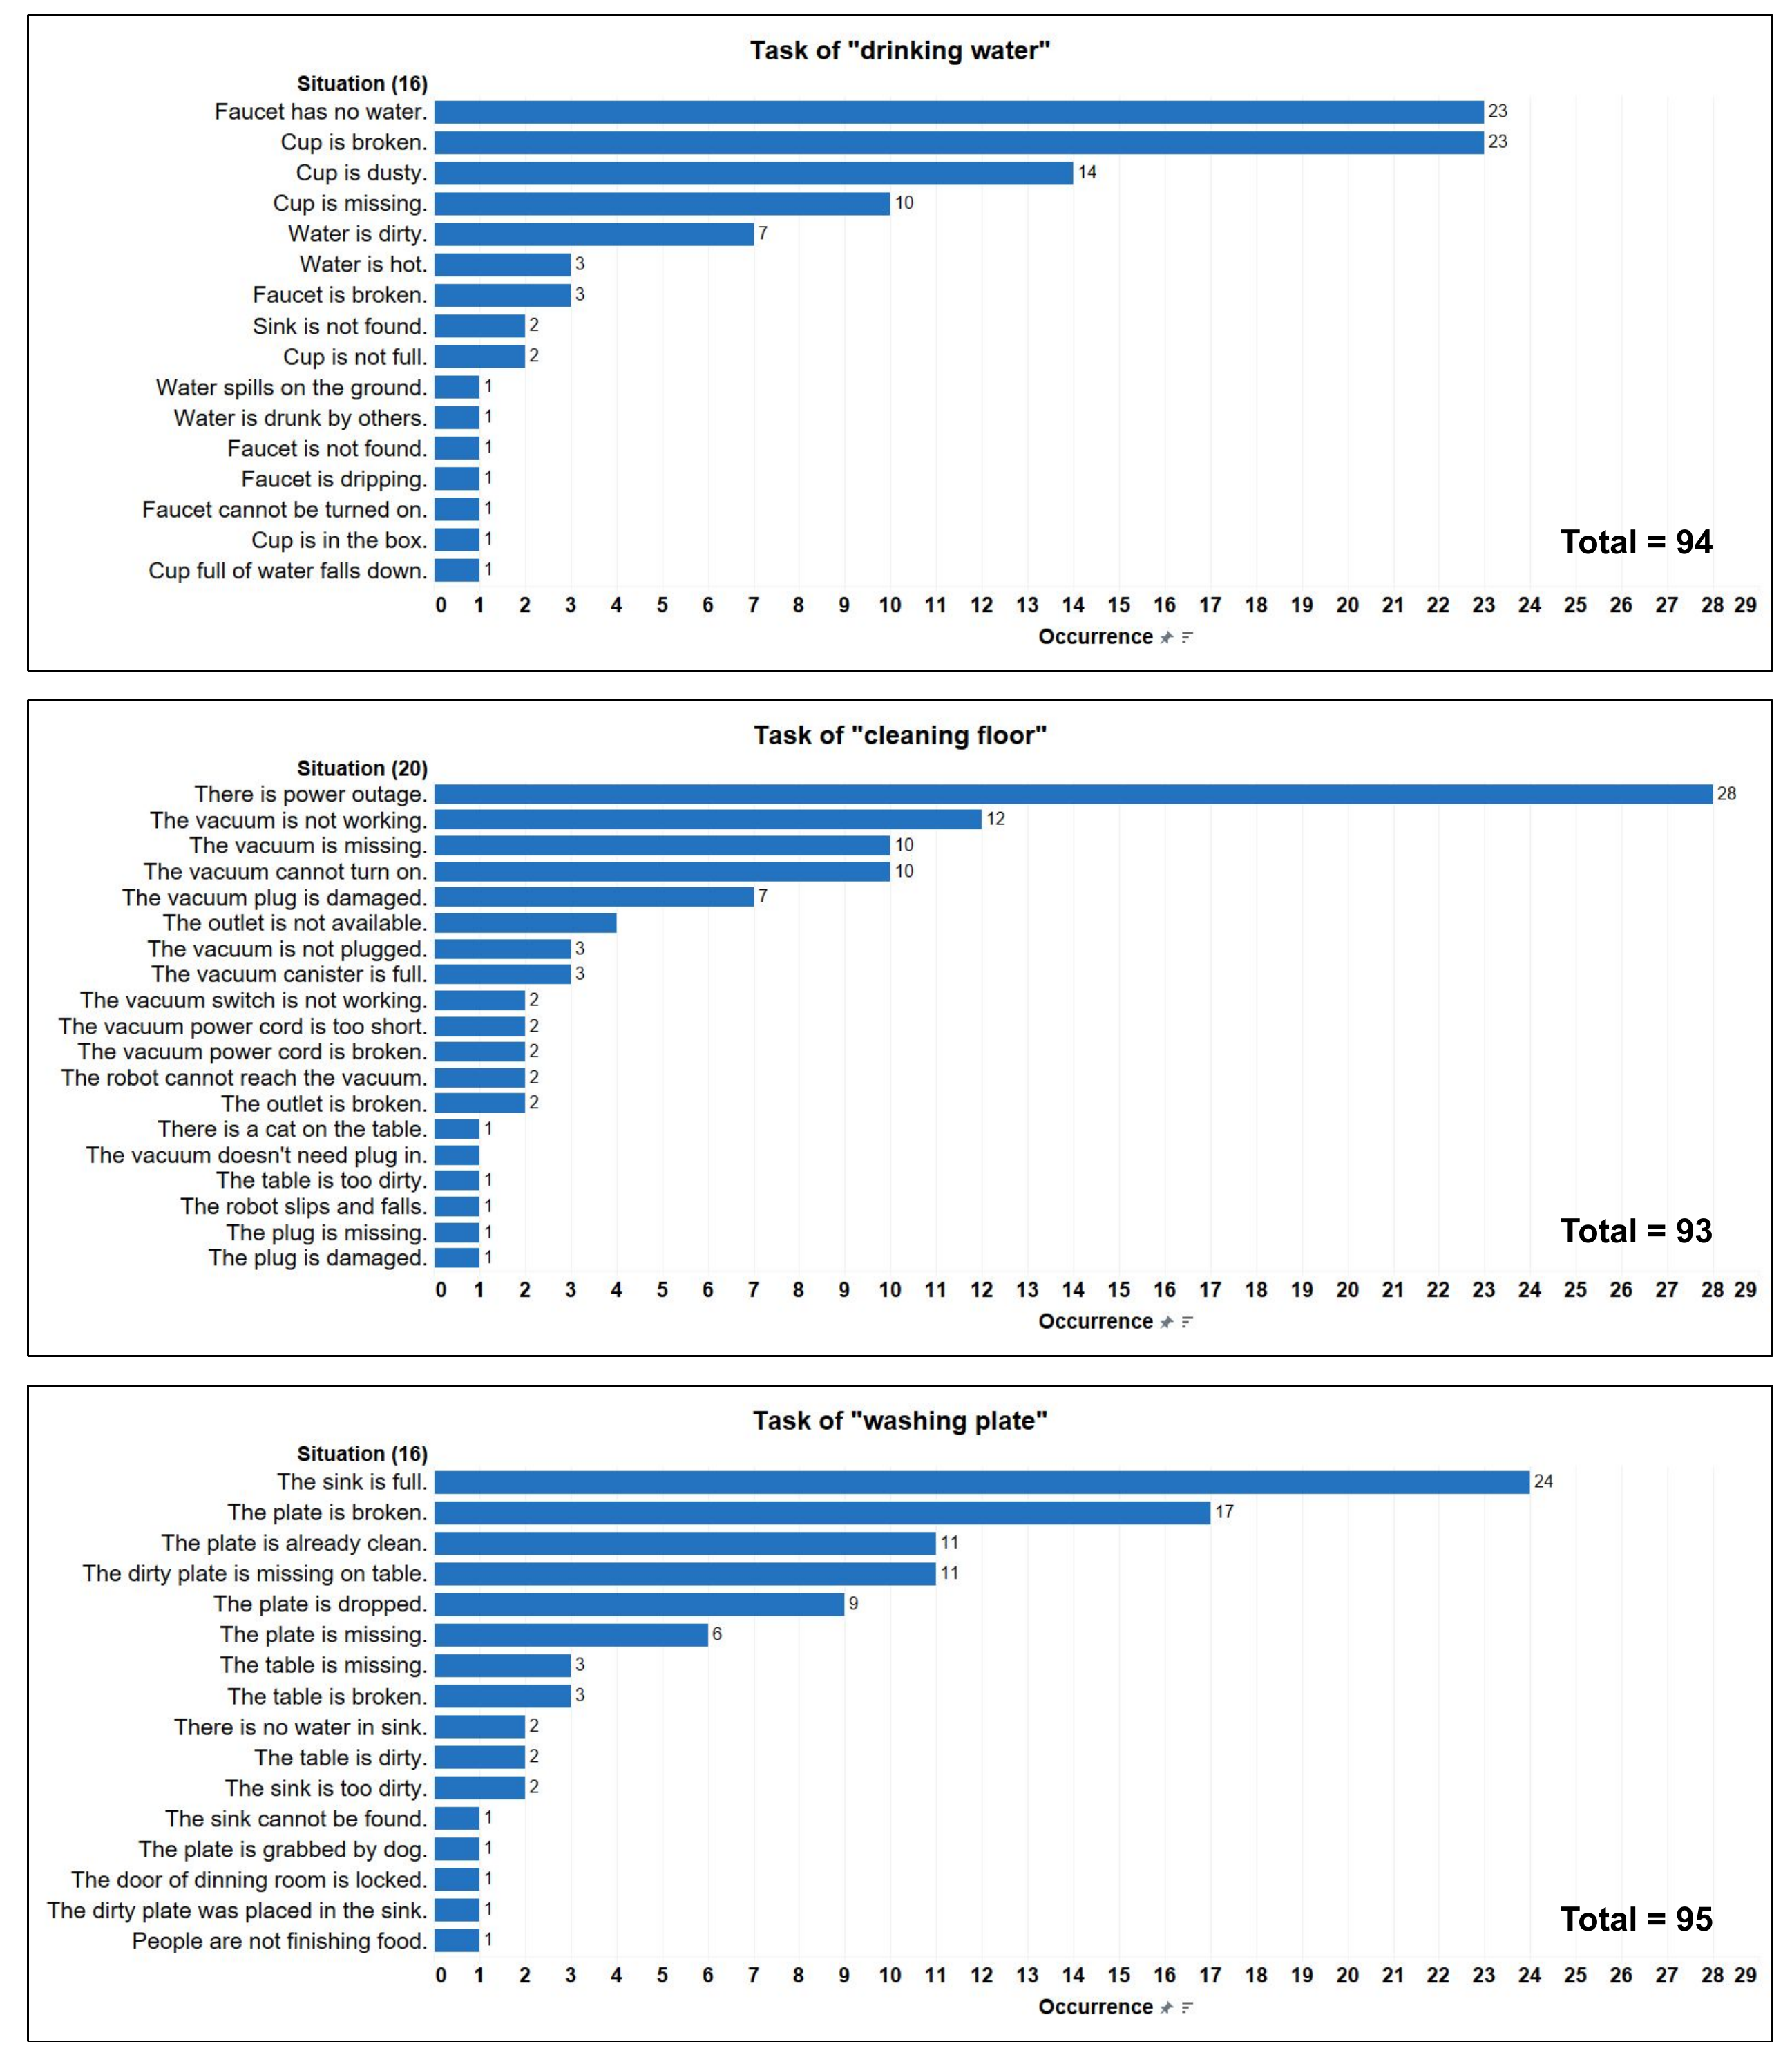}
\caption{
\textbf{Top:} Details of situations in the task of ``drinking water'';
\textbf{Middle:} Details of situations in the task of ``cleaning floor'';
\textbf{Bottom:} Details of situations in the task of ``washing plate'';
\textit{x-axis} reflects the occurrence of each \textit{distinguishable situations}, and \textit{y-axis} represents each distinguishable situations, respectively.
(X) in the top left corner of each subfigure represents the number of distinguishable situations in each task.
Total = X indicates the number of situations in each task.
}\label{fig:situation456}
\end{figure}

\section{Object Library for Simulation}
For simulating dining tasks, we extracted 86 objects (e.g., cup, burger, folk, table, and chair) from an existing dataset~\cite{huang2022language}.
Fig.~\ref{fig:object} shows these objects, which is categorized into five groups: utensil, appliance, furniture, food, and beverage.
From the figure, we can see that the category ``utensil'' contains the greatest number of objects (i.e., 29), while the category ``beverage'' contains the fewest ones (i.e., 8).

% editable figure link: None
\begin{figure}[!hpt]
\centering
\includegraphics[width=1\columnwidth]{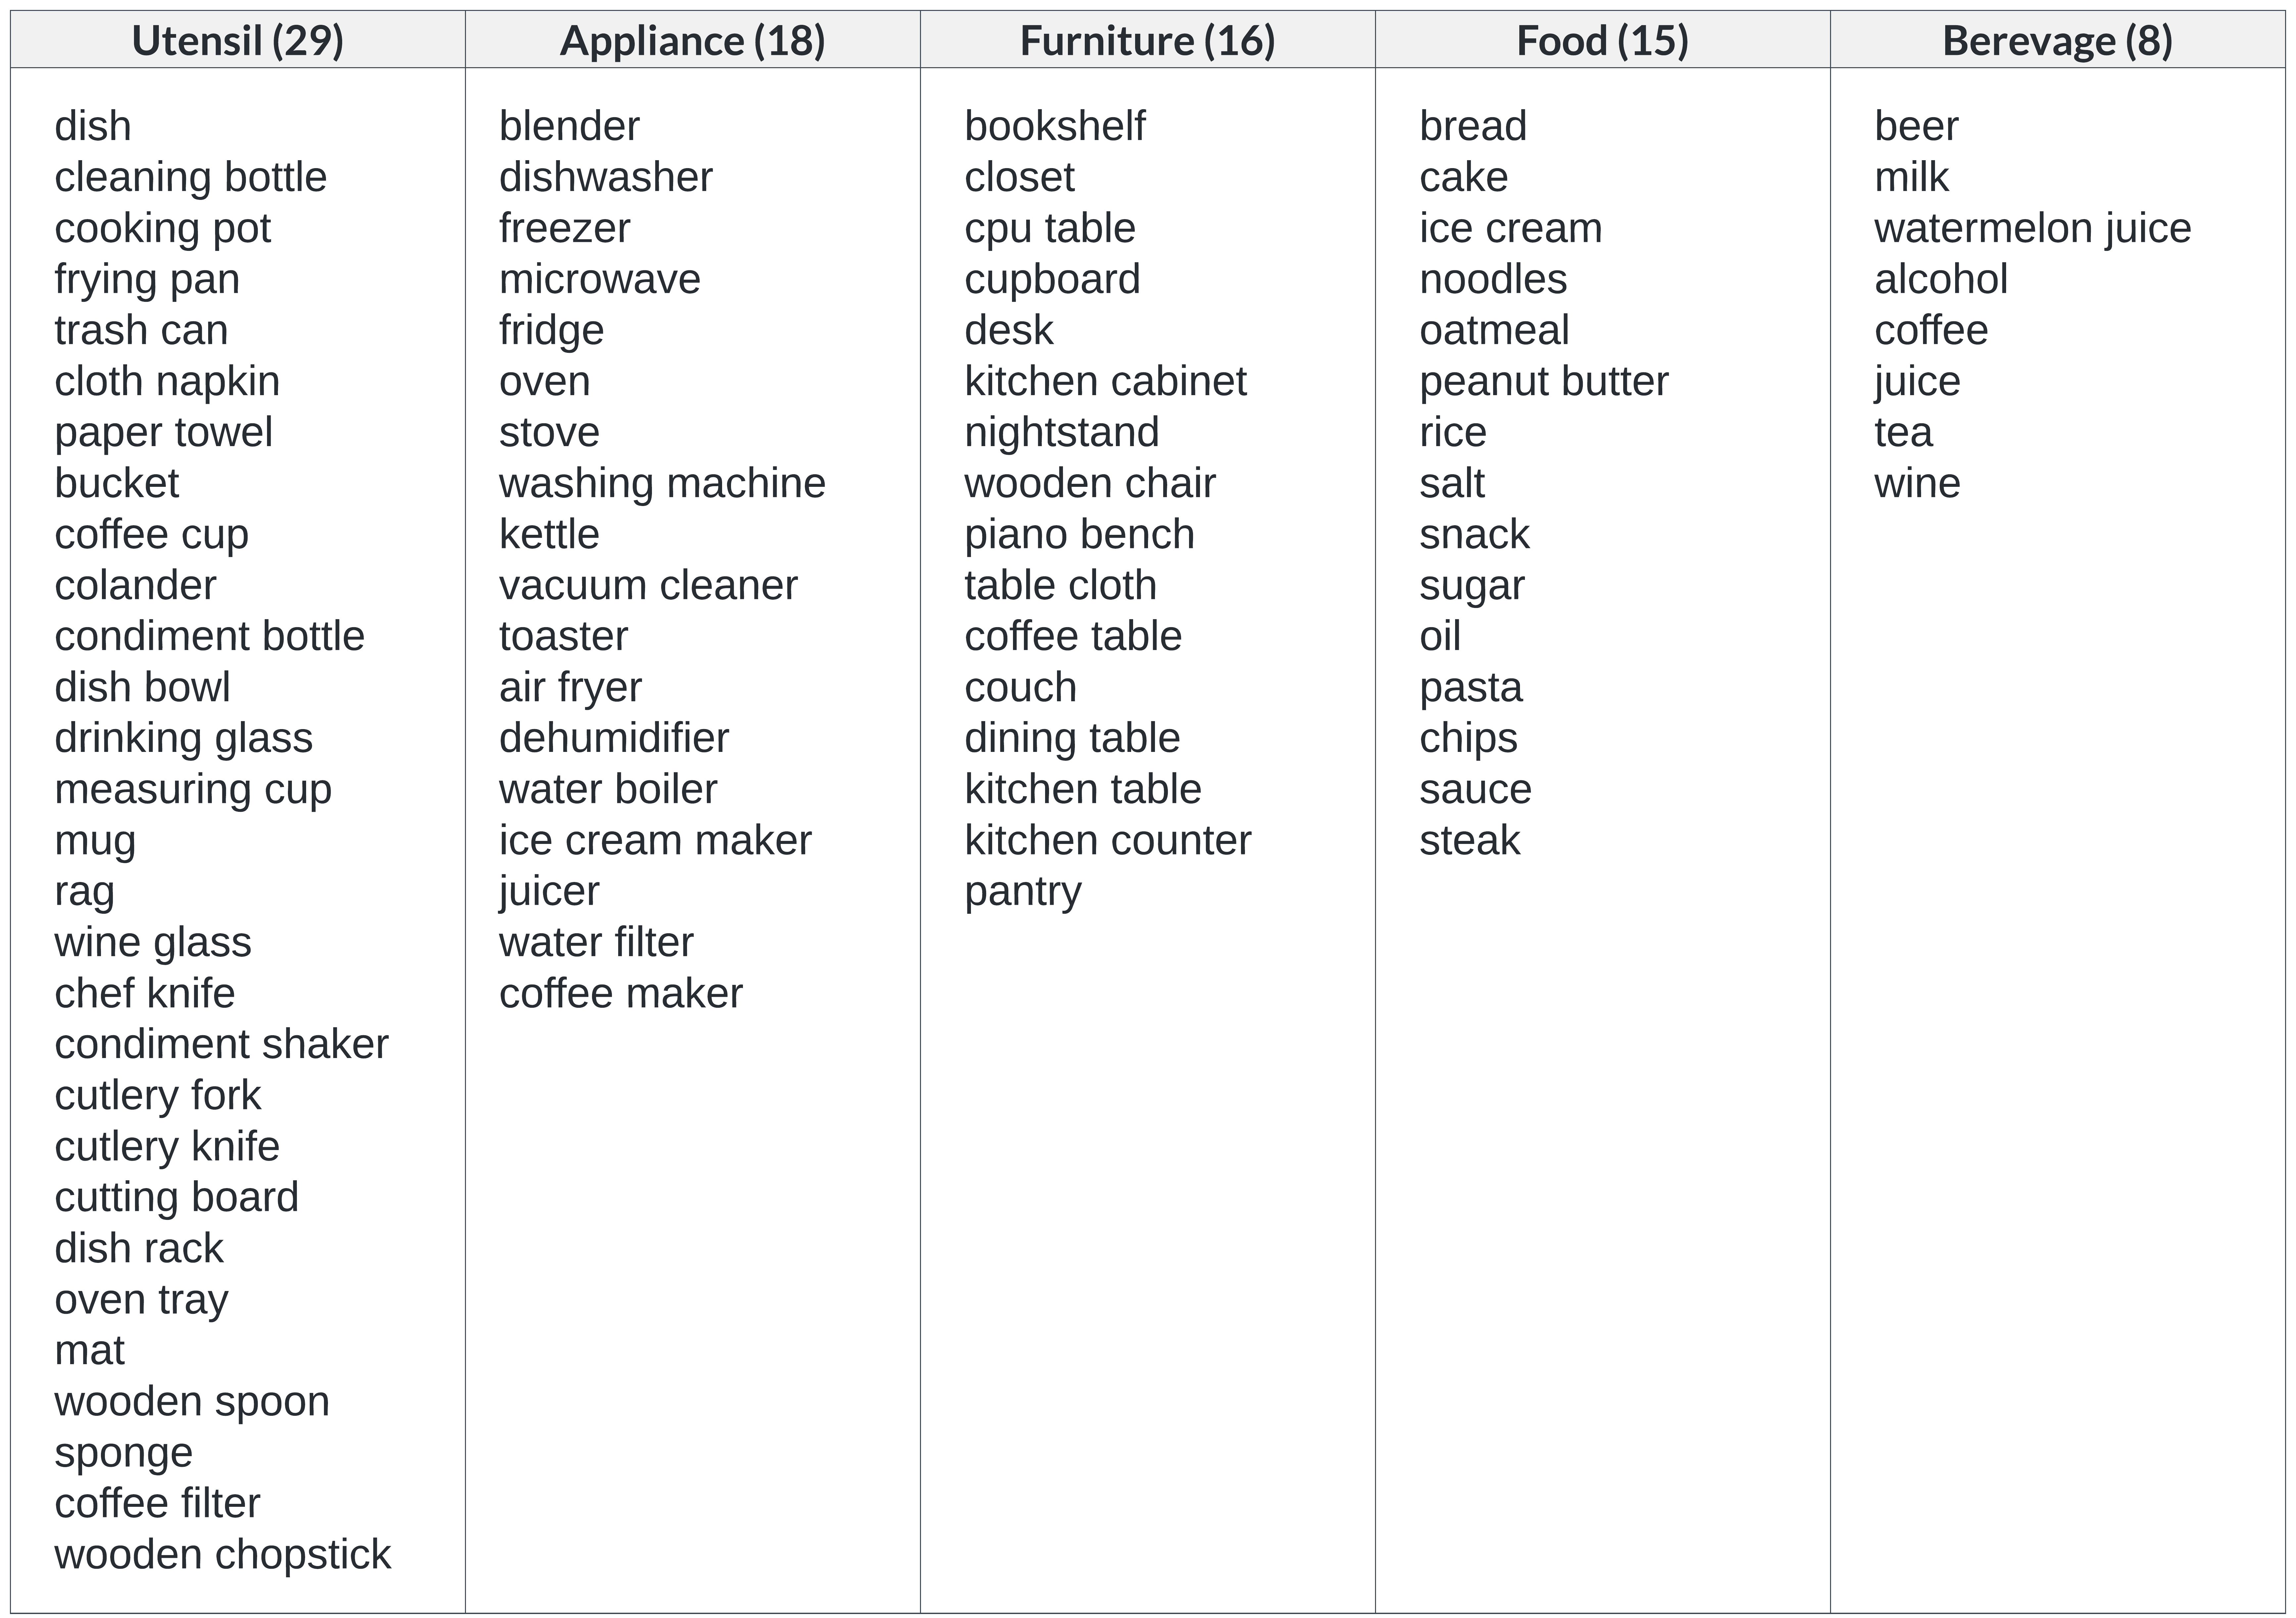}
\caption{For simulating dining tasks, we extracted 86 objects from an existing dataset~\cite{huang2022language}.
These objects are categorized into five groups: utensil, appliance, furniture, food, and beverage, with (X) representing the number of objects in each group.
}\label{fig:object}
\end{figure}

\section{Closed-World Task Planners in PDDL}
For each task in the evaluation, we developed a closed-world task planner in PDDL.
PDDL, an action-centered language, is designed to formalize Artificial Intelligence (AI) planning problems, allowing for a more direct comparison of planning algorithms and implementations~\cite{aeronautiques1998pddl}.
Fig.~\ref{fig:planner} shows a task planner for the task of ``drinking water'', which consists of a domain file (\textbf{upper}) and a problem file (\textbf{lower}).
In the upper subfigure, a set of predicates (e.g., \texttt{cup\_at}) and a set of actions (e.g., \texttt{fill}) are predefined, where an action is defined by its preconditions and effects.
For example, one of preconditions for action \texttt{fill} is \texttt{(cup\_is\_held ?c) $\wedge$ (cup\_is\_empty ?c)}, and the action effect is \texttt{(cup\_is\_filled ?c)}.
In the lower subfigure, a task problem is defined by an initial state and a goal state (i.e., a user is satisfied and the faucet is turned off.)
A task plan for drinking water is generated after inputting these two files into a solver\footnote{The solver is accessible at \url{http://editor.planning.domains/}}, as shown below:
\vspace{1em}
\begin{center}
\begin{minipage}{0.55\textwidth}
\footnotesize{
\begin{Verbatim}[frame=lines, label=Task Plan for Drinking Water ,labelposition=topline, commandchars=\\\{\}]
\vspace{0.1em}
S1: (walk rob dining kitchen)
S2: (find_faucet rob faucet_0 kitchen)
S3: (find_cup rob cup_1 kitchen)
S4: (hold rob cup_1 kitchen)
S5: (turnon rob faucet_0 kitchen)
S6: (fill rob cup_1 faucet_0 kitchen)
S7: (turnoff rob faucet_0 kitchen)
S8: (walk rob kitchen dining)
S9: (place rob cup_1 table_0 dining)
S10: (done cup_1 person_1)
\vspace{0.1em}
\end{Verbatim}
}
\end{minipage}
\end{center}
\vspace{1em}
% A situation that prevents the generated task plan from executing will introduce a new action precondition.
% The common sense extracted from Knowledge Acquirer will be added into the action effect.

% editable figure link: https://docs.google.com/drawings/d/18-hrH7g9BXPa_tAx7lpEEb0xiEMVEmcLCfN-mmDJ2L4/edit
\begin{figure}[t]
\centering
\includegraphics[width=1\columnwidth]{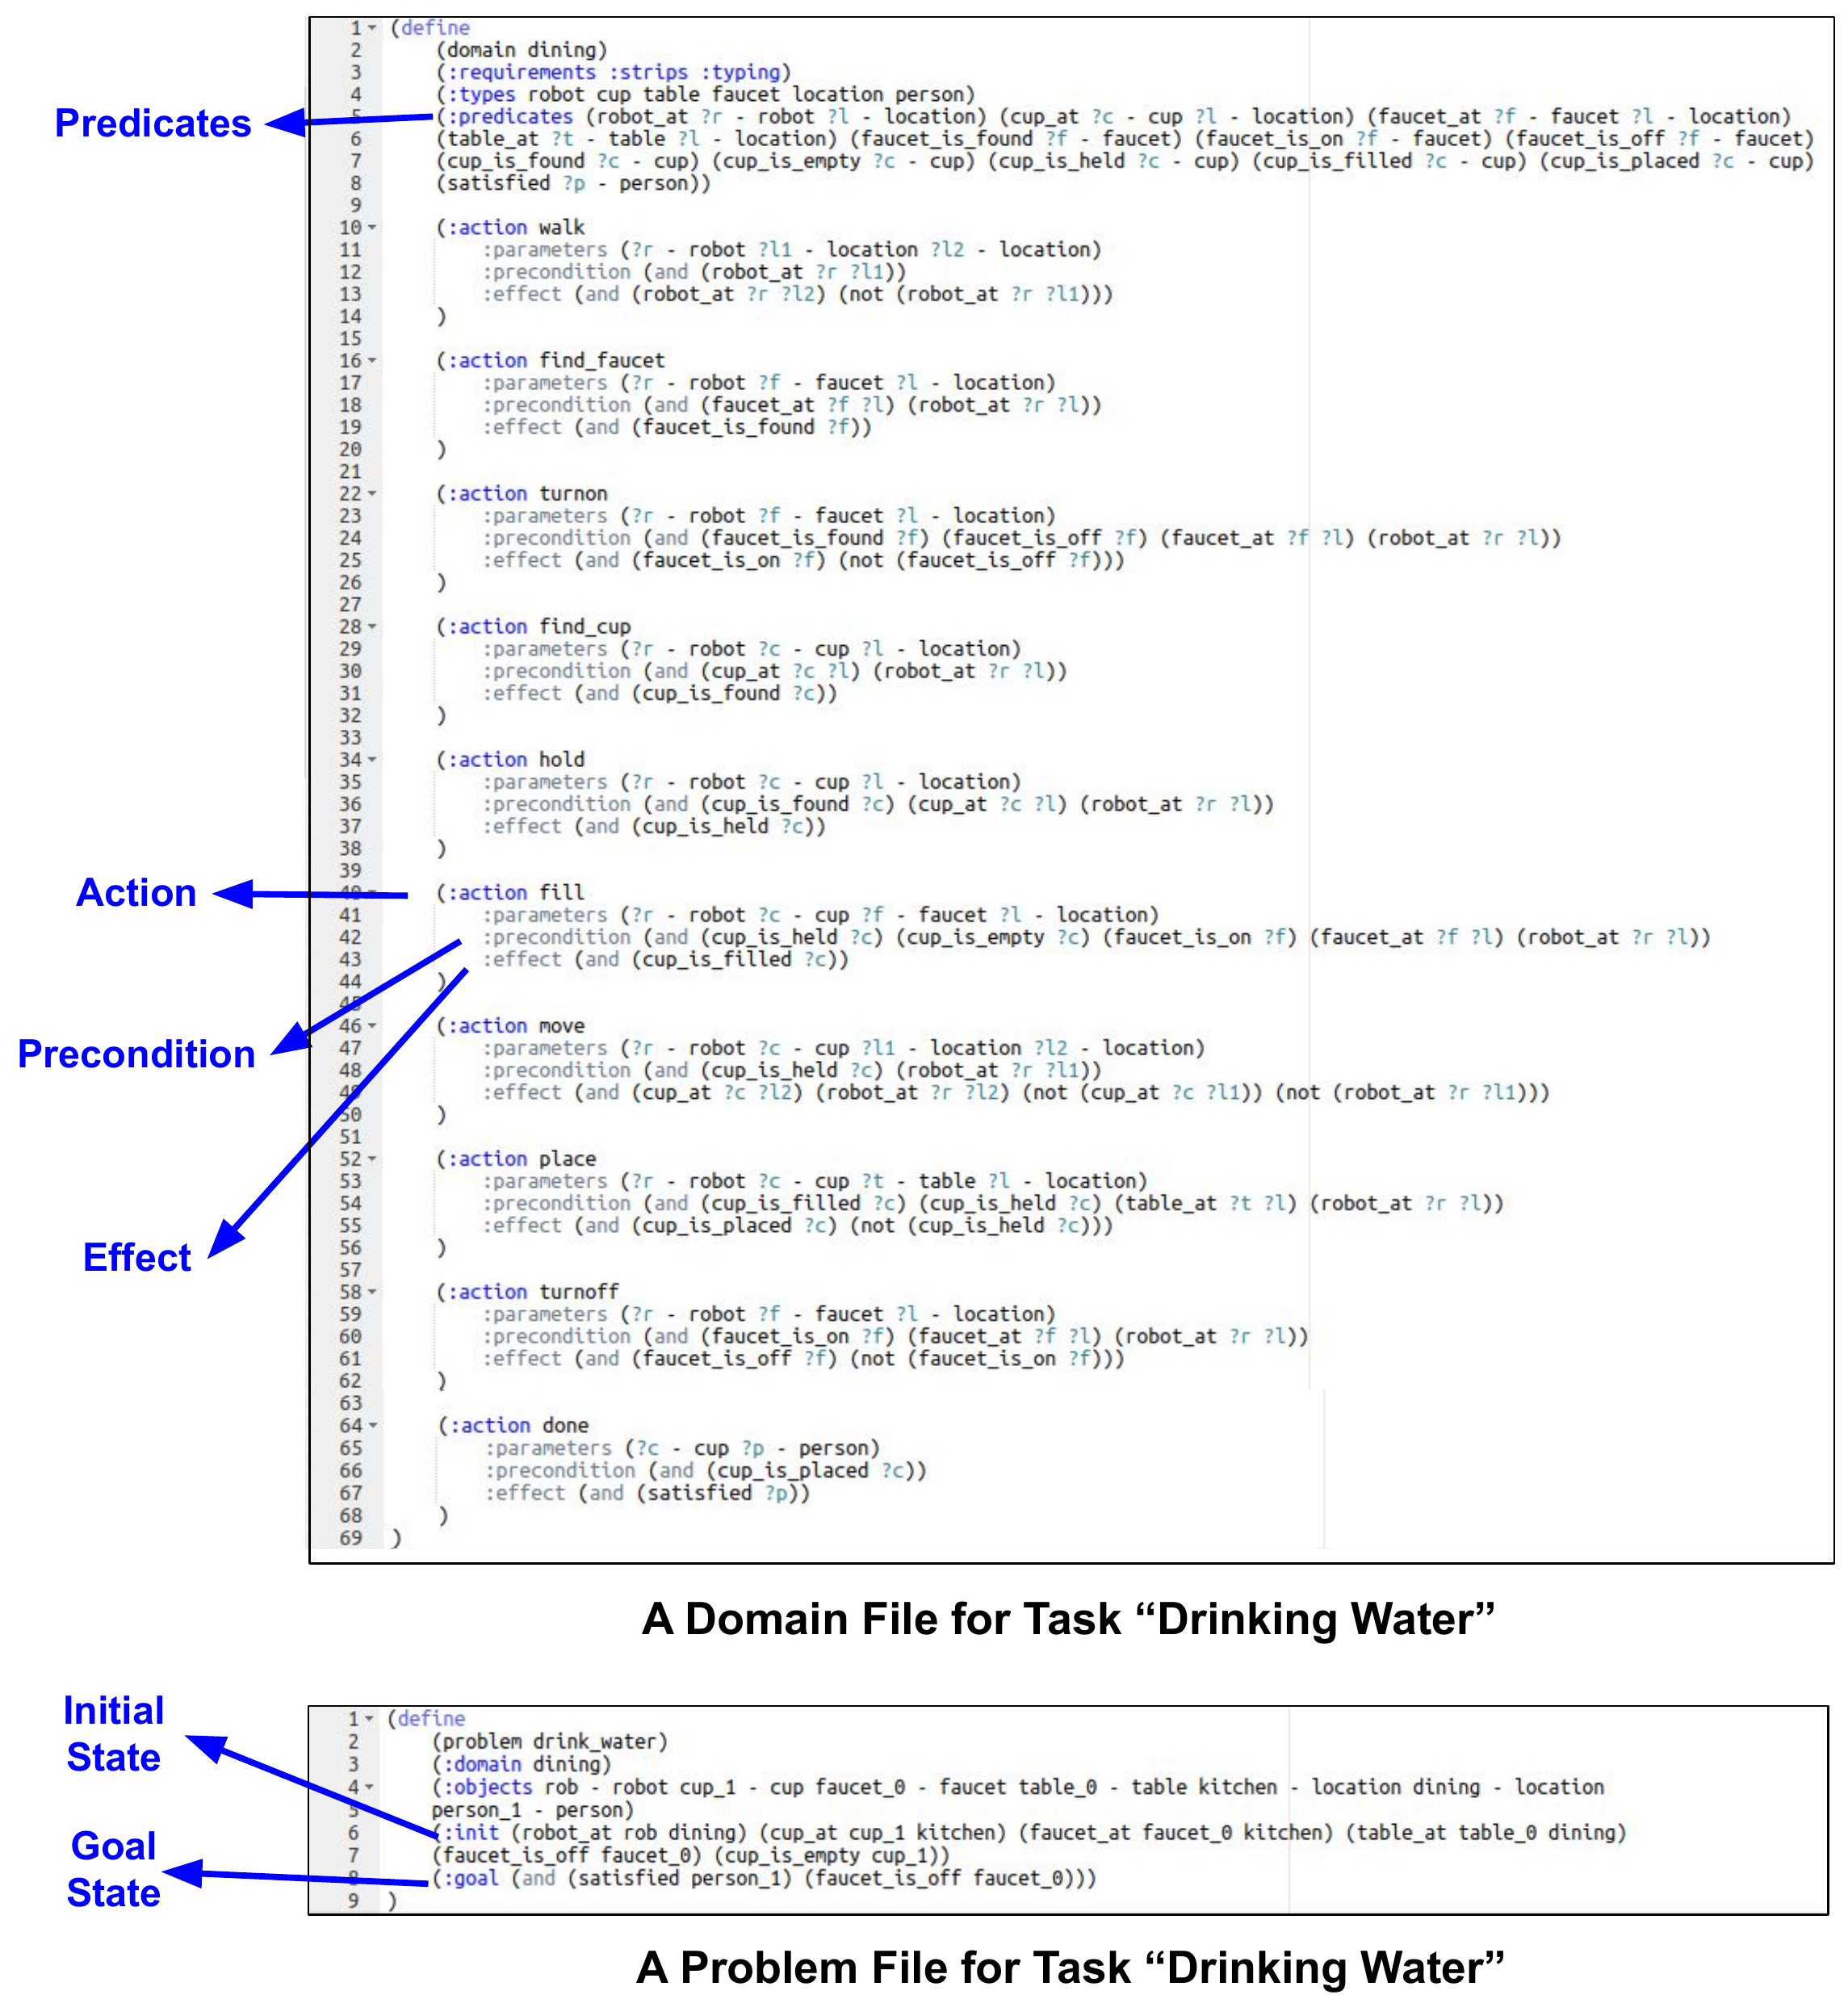}
\caption{A closed-world task planner in PDDL for the task of ``drinking water'', consisting of a domain file (\textbf{upper}) and a problem file (\textbf{lower}).
In the upper subfigure, a set of predicates and a set of actions are predefined, where an action is defined by its preconditions and effects.
In the lower subfigure, a task problem is defined by an initial state and a goal state.
}\label{fig:planner}
\end{figure}

\section{Prompt Design}
Fig.~\ref{fig:templates} shows three examples for prompt construction based on our Templates 1-3, respectively.
In the figure, the interface, called Playground\footnote{The playground of GPT-3 is accessible at \url{https://beta.openai.com/playground}.}, is intended for testing GPT-3 online, where a user can text a prompt in the blank, and customize the hyperparameters of GPT-3 (e.g., model).
In our case, we use the \textit{text-davinci-002} model, which is the most capable engine.
The prompt for Plan Monitor (PM) is constructed based on Template 1, where PM evaluates if the current task plan is feasible or not.
In the \textbf{top} figure, we can know an action precondition that ``one cannot fill a broken cup with water'' according to the common sense from GPT-3.
The prompts for Knowledge Acquirer (KA) are constructed based on Template 2 and Template 3, where KA extracts common sense to augment the classical task planner.
In these two figures (\textbf{middle} and \textbf{bottom}), we can know that common sense that ``one can use a bowl for drinking water'' can be added into an action effect, according to the common sense from GPT-3.
% The most prevalent settings for prompting are either \textit{zero-shot} (ZS) or \textit{few-shot} (FS).
% In the top and bottom figures, a ZS prompt is adopted, which directly describes the task without providing any demonstrations.
% In the middle figure, a FS prompt is adopted, where eight examples are provided to instruct GPT-3 what pattern to follow by feeding it examples of desired inputs and outputs.

% editable figure link: https://docs.google.com/drawings/d/1FZjSdyIowlnxHezKasDB1taVwIr-Agm0j4dR9ljHj88/edit
\begin{figure}[t]
\centering
\includegraphics[width=0.9\columnwidth]{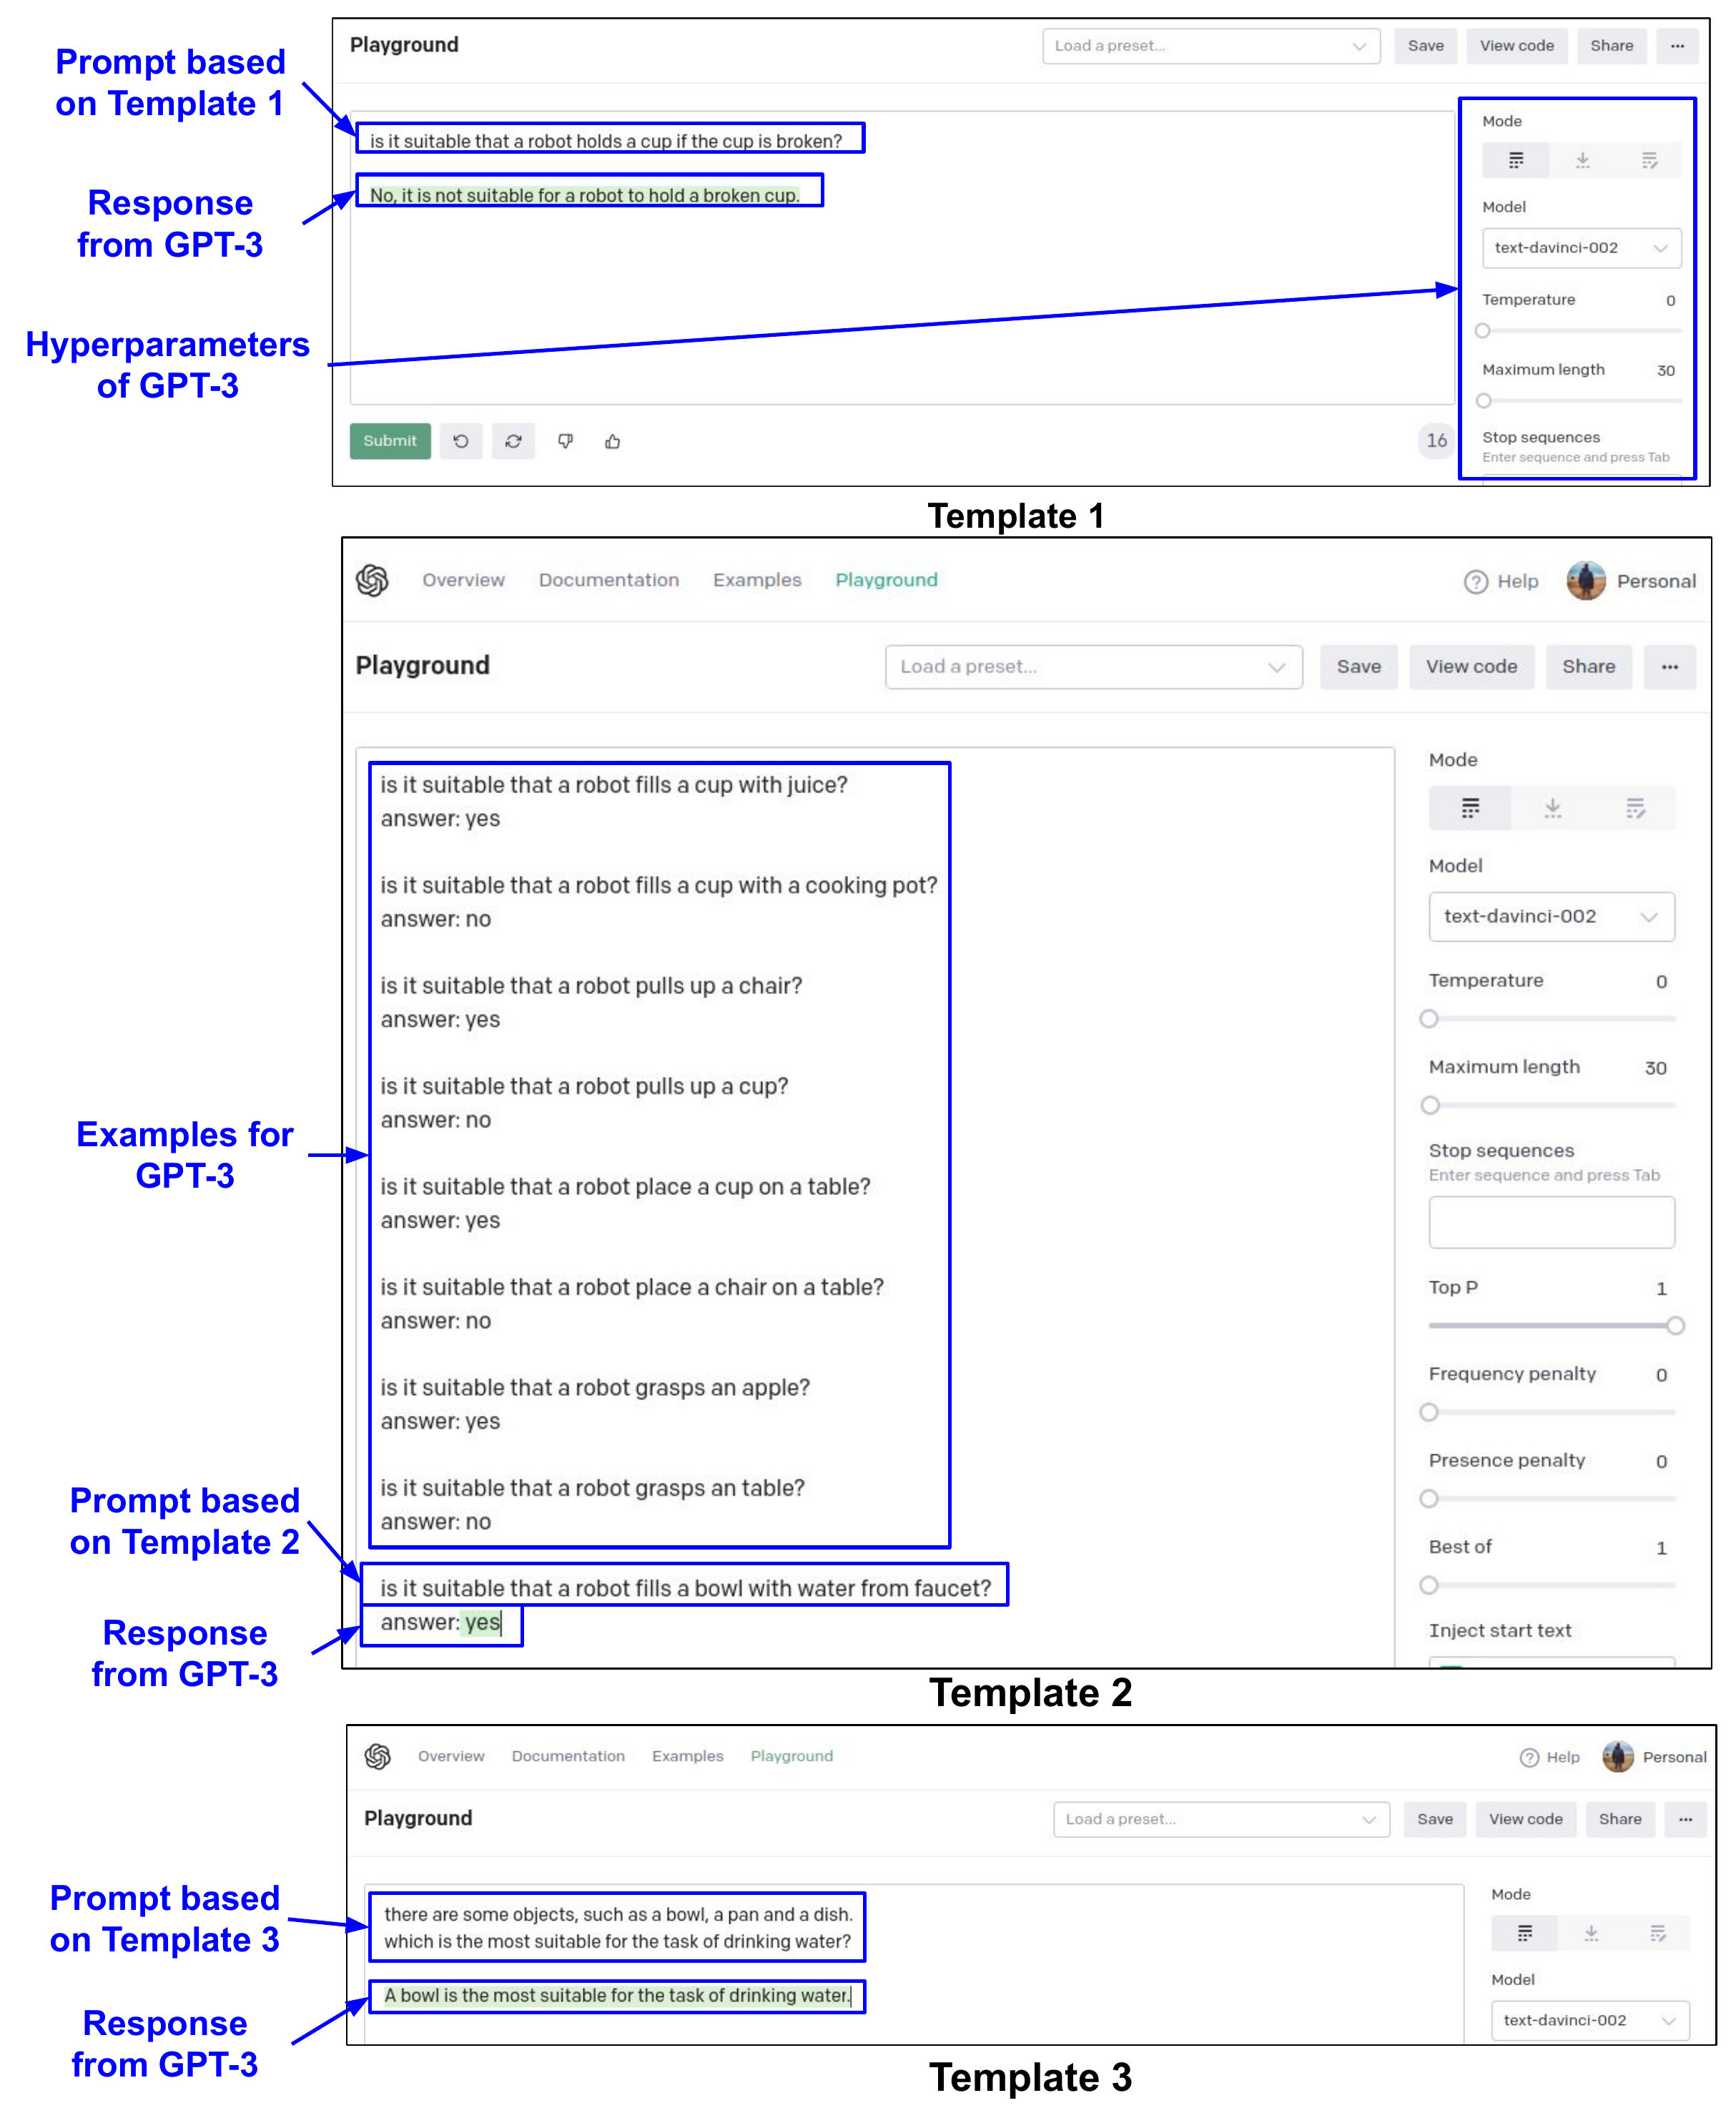}
\caption{Three examples for prompt construction based on Templates 1-3.
}\label{fig:templates}
\end{figure}

\textcolor{red}{On the above note, it would also make sense for authors to include more examples of success and failure cases, for
all baselines, (perhaps in appendix) and analyze these examples.}
